# Supplementary material for: Mode-Suppression: A Simple, Stable and Scalable Chunk-Sharing Algorithm for P2P Networks
Source: arXiv:1904.04191 source file (2019-04-08)
Supplement: Supplementary file 1 [file 9.appendix.tex]

\appendix
\label{sec:appendix}
